# Supplementary material for: YFlows: Systematic Dataflow Exploration and Code Generation for Efficient Neural Network Inference using SIMD Architectures on CPUs
Source: arXiv:2310.00574 source file (2023-11-23)
Supplement: Supplementary file 1 [file appendix.tex]

\section*{Appendix 1: Example Assembly Code Snippet under Basic OS Dataflow, Binarized Implementation}

\scriptsize\begin{verbatim}
            .......
 a54:	937d7cc6 	sbfiz	x6, x6, #3, #32
 a58:	3ce66b40 	ldr	q0, [x26, x6]
 a5c:	6e211c00 	eor	v0.16b, v0.16b, v1.16b
 a60:	4e205800 	cnt	v0.16b, v0.16b
 a64:	4e31b800 	addv	b0, v0.16b
 a68:	0e013c06 	umov	w6, v0.b[0]
 a6c:	4b060366 	sub	w6, w27, w6
 a70:	0b060400 	add	w0, w0, w6, lsl #1
 a74:	7101bc3f 	cmp	w1, #0x6f
 a78:	5400018c 	b.gt	aa8 <main+0x1e8>
 a7c:	0b020306 	add	w6, w24, w2
 a80:	3dc001c1 	ldr	q1, [x14]
 a84:	13067cc6 	asr	w6, w6, #6
 a88:	937d7cc6 	sbfiz	x6, x6, #3, #32
 a8c:	3ce66b40 	ldr	q0, [x26, x6]
 a90:	6e211c00 	eor	v0.16b, v0.16b, v1.16b
 a94:	4e205800 	cnt	v0.16b, v0.16b
 a98:	4e31b800 	addv	b0, v0.16b
 a9c:	0e013c06 	umov	w6, v0.b[0]
 aa0:	4b060366 	sub	w6, w27, w6
 aa4:	0b060400 	add	w0, w0, w6, lsl #1
 aa8:	7101bc9f 	cmp	w4, #0x6f
 aac:	5400018c 	b.gt	adc <main+0x21c>
 ab0:	0b020266 	add	w6, w19, w2
 ab4:	3dc001a1 	ldr	q1, [x13]
 ab8:	13067cc6 	asr	w6, w6, #6
 abc:	937d7cc6 	sbfiz	x6, x6, #3, #32
 ac0:	3ce66b40 	ldr	q0, [x26, x6]
 ac4:	6e211c00 	eor	v0.16b, v0.16b, v1.16b
 ac8:	4e205800 	cnt	v0.16b, v0.16b
 acc:	4e31b800 	addv	b0, v0.16b
 ad0:	0e013c06 	umov	w6, v0.b[0]
 ad4:	4b060366 	sub	w6, w27, w6
 ad8:	0b060400 	add	w0, w0, w6, lsl #1
 adc:	7101bcff 	cmp	w7, #0x6f
 ae0:	54000508 	b.hi	b80 <main+0x2c0>  // b.pmore
 ae4:	f101bc7f 	cmp	x3, #0x6f
 ae8:	54000188 	b.hi	b18 <main+0x258>  // b.pmore
 aec:	0b0202a6 	add	w6, w21, w2
 af0:	3dc00181 	ldr	q1, [x12]
 af4:	13067cc6 	asr	w6, w6, #6
 af8:	937d7cc6 	sbfiz	x6, x6, #3, #32
 afc:	3ce66b40 	ldr	q0, [x26, x6]
 b00:	6e211c00 	eor	v0.16b, v0.16b, v1.16b
 b04:	4e205800 	cnt	v0.16b, v0.16b
 b08:	4e31b800 	addv	b0, v0.16b
 b0c:	0e013c06 	umov	w6, v0.b[0]
 b10:	4b060366 	sub	w6, w27, w6
 b14:	0b060400 	add	w0, w0, w6, lsl #1
 b18:	7101bc3f 	cmp	w1, #0x6f
 b1c:	5400018c 	b.gt	b4c <main+0x28c>
 b20:	0b0202c6 	add	w6, w22, w2
 b24:	3dc00161 	ldr	q1, [x11]
 b28:	13067cc6 	asr	w6, w6, #6
 b2c:	937d7cc6 	sbfiz	x6, x6, #3, #32
 b30:	3ce66b40 	ldr	q0, [x26, x6]
 b34:	6e211c00 	eor	v0.16b, v0.16b, v1.16b
 b38:	4e205800 	cnt	v0.16b, v0.16b
 b3c:	4e31b800 	addv	b0, v0.16b
 b40:	0e013c06 	umov	w6, v0.b[0]
 b44:	4b060366 	sub	w6, w27, w6
 b48:	0b060400 	add	w0, w0, w6, lsl #1
 b4c:	7101bc9f 	cmp	w4, #0x6f
 b50:	5400018c 	b.gt	b80 <main+0x2c0>
 b54:	0b020246 	add	w6, w18, w2
 b58:	3dc00141 	ldr	q1, [x10]
 b5c:	13067cc6 	asr	w6, w6, #6
 b60:	937d7cc6 	sbfiz	x6, x6, #3, #32
 b64:	3ce66b40 	ldr	q0, [x26, x6]
 b68:	6e211c00 	eor	v0.16b, v0.16b, v1.16b
 b6c:	4e205800 	cnt	v0.16b, v0.16b
 b70:	4e31b800 	addv	b0, v0.16b
 b74:	0e013c06 	umov	w6, v0.b[0]
 b78:	4b060366 	sub	w6, w27, w6
 b7c:	0b060400 	add	w0, w0, w6, lsl #1
 b80:	d376d466 	lsl	x6, x3, #10
 b84:	93407c00 	sxtw	x0, w0
 b88:	11000484 	add	w4, w4, #0x1
 b8c:	11020042 	add	w2, w2, #0x80
 b90:	91000463 	add	x3, x3, #0x1
 b94:	f8266900 	str	x0, [x8, x6]
 b98:	7101c83f 	cmp	w1, #0x72
 b9c:	540005a0 	b.eq	c50 <main+0x390>  // b.none
 ba0:	7101bc3f 	cmp	w1, #0x6f
 ba4:	52800000 	mov	w0, #0x0                   	// #0
 ba8:	7a40d8a4 	ccmp	w5, #0x0, #0x4, le
 bac:	54fff380 	b.eq	a1c <main+0x15c>  // b.none
 bb0:	51040040 	sub	w0, w2, #0x100
 bb4:	11000421 	add	w1, w1, #0x1
 bb8:	3dc00281 	ldr	q1, [x20]
 bbc:	13067c00 	asr	w0, w0, #6
 bc0:	7101bc3f 	cmp	w1, #0x6f
 bc4:	937d7c00 	sbfiz	x0, x0, #3, #32
 bc8:	7a40d8a4 	ccmp	w5, #0x0, #0x4, le
 bcc:	3ce06b40 	ldr	q0, [x26, x0]
 bd0:	6e211c00 	eor	v0.16b, v0.16b, v1.16b
 bd4:	4e205800 	cnt	v0.16b, v0.16b
 bd8:	4e31b800 	addv	b0, v0.16b
 bdc:	0e013c00 	umov	w0, v0.b[0]
 be0:	4b000360 	sub	w0, w27, w0
 be4:	531f7800 	lsl	w0, w0, #1
 be8:	54fff220 	b.eq	a2c <main+0x16c>  // b.none
 bec:	51020046 	sub	w6, w2, #0x80
 bf0:	7101bc9f 	cmp	w4, #0x6f
 bf4:	3dc00221 	ldr	q1, [x17]
 bf8:	13067cc6 	asr	w6, w6, #6
 bfc:	7a40d8a4 	ccmp	w5, #0x0, #0x4, le
 c00:	937d7cc6 	sbfiz	x6, x6, #3, #32
 c04:	3ce66b40 	ldr	q0, [x26, x6]
 c08:	6e211c00 	eor	v0.16b, v0.16b, v1.16b
 c0c:	4e205800 	cnt	v0.16b, v0.16b
 c10:	4e31b800 	addv	b0, v0.16b
 c14:	0e013c06 	umov	w6, v0.b[0]
 c18:	4b060366 	sub	w6, w27, w6
 c1c:	0b060400 	add	w0, w0, w6, lsl #1
 c20:	54fff0c0 	b.eq	a38 <main+0x178>  // b.none
 c24:	13067c46 	asr	w6, w2, #6
 c28:	3dc00201 	ldr	q1, [x16]
 c2c:	937d7cc6 	sbfiz	x6, x6, #3, #32
 c30:	3ce66b40 	ldr	q0, [x26, x6]
 c34:	6e211c00 	eor	v0.16b, v0.16b, v1.16b
 c38:	4e205800 	cnt	v0.16b, v0.16b
 c3c:	4e31b800 	addv	b0, v0.16b
 c40:	0e013c06 	umov	w6, v0.b[0]
 c44:	4b060366 	sub	w6, w27, w6
 c48:	0b060400 	add	w0, w0, w6, lsl #1
            .......
\end{verbatim}
\newpage
\section*{Appendix 2: Example Assembly Code Snippet under Extended OS Dataflow, Binarized Implementation}

\scriptsize\begin{verbatim}
            .......
 8c0:	a9b97bfd 	stp	x29, x30, [sp, #-112]!
 8c4:	90000001 	adrp	x1, 0 <_init-0x7d8>
 8c8:	913a8021 	add	x1, x1, #0xea0
 8cc:	910003fd 	mov	x29, sp
 8d0:	90000000 	adrp	x0, 0 <_init-0x7d8>
 8d4:	913aa000 	add	x0, x0, #0xea8
 8d8:	a90153f3 	stp	x19, x20, [sp, #16]
 8dc:	a9025bf5 	stp	x21, x22, [sp, #32]
 8e0:	f9001bf7 	str	x23, [sp, #48]
 8e4:	6d0427e8 	stp	d8, d9, [sp, #64]
 8e8:	6d052fea 	stp	d10, d11, [sp, #80]
 8ec:	3d801be8 	str	q8, [sp, #96]
 8f0:	97ffffe0 	bl	870 <fopen@plt>
 8f4:	aa0003f6 	mov	x22, x0
 8f8:	d2892000 	mov	x0, #0x4900                	// #18688
 8fc:	f2a00060 	movk	x0, #0x3, lsl #16
 900:	97ffffe4 	bl	890 <malloc@plt>
 904:	aa0003f3 	mov	x19, x0
 908:	d2820000 	mov	x0, #0x1000                	// #4096
 90c:	f2a01960 	movk	x0, #0xcb, lsl #16
 910:	97ffffe0 	bl	890 <malloc@plt>
 914:	aa0003f5 	mov	x21, x0
 918:	d2890000 	mov	x0, #0x4800                	// #18432
 91c:	97ffffdd 	bl	890 <malloc@plt>
 920:	aa0003f4 	mov	x20, x0
 924:	97ffffcb 	bl	850 <clock@plt>
 928:	aa0003f7 	mov	x23, x0
 92c:	3dc0027e 	ldr	q30, [x19]
 930:	d299000e 	mov	x14, #0xc800                	// #51200
 934:	3dc01be8 	ldr	q8, [sp, #96]
 938:	aa1403f1 	mov	x17, x20
 93c:	3dc1c67d 	ldr	q29, [x19, #1808]
 940:	aa1503fe 	mov	x30, x21
 944:	3dc38a7c 	ldr	q28, [x19, #3616]
 948:	d2800012 	mov	x18, #0x0                   	// #0
 94c:	3dc54e7b 	ldr	q27, [x19, #5424]
 950:	52870010 	mov	w16, #0x3800                	// #14336
 954:	3dc7127a 	ldr	q26, [x19, #7232]
 958:	5287200f 	mov	w15, #0x3900                	// #14592
 95c:	3dc8d679 	ldr	q25, [x19, #9040]
 960:	f2a0002e 	movk	x14, #0x1, lsl #16
 964:	4ebe1fc7 	mov	v7.16b, v30.16b
 968:	aa1e03ed 	mov	x13, x30
 96c:	4ebd1fa6 	mov	v6.16b, v29.16b
 970:	5280000b 	mov	w11, #0x0                   	// #0
 974:	4ebc1f85 	mov	v5.16b, v28.16b
 978:	5280000c 	mov	w12, #0x0                   	// #0
 97c:	4ebb1f64 	mov	v4.16b, v27.16b
 980:	4eba1f43 	mov	v3.16b, v26.16b
 984:	4eb91f22 	mov	v2.16b, v25.16b
 988:	ad405e38 	ldp	q24, q23, [x17]
 98c:	ad415636 	ldp	q22, q21, [x17, #32]
 990:	ad424e34 	ldp	q20, q19, [x17, #64]
 994:	ad434632 	ldp	q18, q17, [x17, #96]
 998:	3dc02230 	ldr	q16, [x17, #128]
 99c:	d503201f 	nop
 9a0:	11401d66 	add	w6, w11, #0x7, lsl #12
 9a4:	0b10016b 	add	w11, w11, w16
 9a8:	2a0c03e1 	mov	w1, w12
 9ac:	11000980 	add	w0, w12, #0x2
 9b0:	13077cc6 	asr	w6, w6, #7
 9b4:	13077d6c 	asr	w12, w11, #7
 9b8:	4b0100c6 	sub	w6, w6, w1
 9bc:	4b010181 	sub	w1, w12, w1
 9c0:	53196000 	lsl	w0, w0, #7
 9c4:	531960c6 	lsl	w6, w6, #7
 9c8:	aa0d03e5 	mov	x5, x13
 9cc:	53196027 	lsl	w7, w1, #7
 9d0:	110200ca 	add	w10, w6, #0x80
 9d4:	110200e9 	add	w9, w7, #0x80
 9d8:	0b0f0008 	add	w8, w0, w15
 9dc:	d503201f 	nop
 9e0:	13067c02 	asr	w2, w0, #6
 9e4:	11020001 	add	w1, w0, #0x80
 9e8:	6e271f09 	eor	v9.16b, v24.16b, v7.16b
 9ec:	0b0000e4 	add	w4, w7, w0
 9f0:	937d7c42 	sbfiz	x2, x2, #3, #32
 9f4:	13067c21 	asr	w1, w1, #6
 9f8:	6e261eff 	eor	v31.16b, v23.16b, v6.16b
 9fc:	13067c84 	asr	w4, w4, #6
 a00:	937d7c21 	sbfiz	x1, x1, #3, #32
 a04:	0b000123 	add	w3, w9, w0
 a08:	3ce26a67 	ldr	q7, [x19, x2]
 a0c:	937d7c84 	sbfiz	x4, x4, #3, #32
 a10:	4e205929 	cnt	v9.16b, v9.16b
 a14:	13067c63 	asr	w3, w3, #6
 a18:	4e205bff 	cnt	v31.16b, v31.16b
 a1c:	0b0000c2 	add	w2, w6, w0
 a20:	6e261f00 	eor	v0.16b, v24.16b, v6.16b
 a24:	937d7c63 	sbfiz	x3, x3, #3, #32
 a28:	6e271ee1 	eor	v1.16b, v23.16b, v7.16b
 a2c:	13067c42 	asr	w2, w2, #6
 a30:	3ce16a66 	ldr	q6, [x19, x1]
 a34:	937d7c42 	sbfiz	x2, x2, #3, #32
 a38:	4e2987ff 	add	v31.16b, v31.16b, v9.16b
 a3c:	0b000141 	add	w1, w10, w0
 a40:	6e271ecb 	eor	v11.16b, v22.16b, v7.16b
 a44:	11040000 	add	w0, w0, #0x100
 a48:	4e205821 	cnt	v1.16b, v1.16b
 a4c:	13067c21 	asr	w1, w1, #6
 a50:	4e205800 	cnt	v0.16b, v0.16b
 a54:	6e261eca 	eor	v10.16b, v22.16b, v6.16b
 a58:	937d7c21 	sbfiz	x1, x1, #3, #32
 a5c:	4e2887ff 	add	v31.16b, v31.16b, v8.16b
 a60:	6e251ea9 	eor	v9.16b, v21.16b, v5.16b
 a64:	4e20596b 	cnt	v11.16b, v11.16b
 a68:	6e241ea8 	eor	v8.16b, v21.16b, v4.16b
 a6c:	4e208420 	add	v0.16b, v1.16b, v0.16b
 a70:	4e20594a 	cnt	v10.16b, v10.16b
 a74:	3ce46a65 	ldr	q5, [x19, x4]
 a78:	4e2b87e1 	add	v1.16b, v31.16b, v11.16b
 a7c:	4e205929 	cnt	v9.16b, v9.16b
 a80:	6e241e9f 	eor	v31.16b, v20.16b, v4.16b
 a84:	4e205908 	cnt	v8.16b, v8.16b
 a88:	4e2a8400 	add	v0.16b, v0.16b, v10.16b
 a8c:	6e251e8b 	eor	v11.16b, v20.16b, v5.16b
 a90:	3ce36a64 	ldr	q4, [x19, x3]
 a94:	4e298421 	add	v1.16b, v1.16b, v9.16b
 a98:	4e205bff 	cnt	v31.16b, v31.16b
 a9c:	6e251e6a 	eor	v10.16b, v19.16b, v5.16b
 aa0:	4e288400 	add	v0.16b, v0.16b, v8.16b
 aa4:	4e20596b 	cnt	v11.16b, v11.16b
 aa8:	6e331c89 	eor	v9.16b, v4.16b, v19.16b
 aac:	6e231e48 	eor	v8.16b, v18.16b, v3.16b
 ab0:	4e3f8421 	add	v1.16b, v1.16b, v31.16b
 ab4:	4e20594a 	cnt	v10.16b, v10.16b
 ab8:	6e221e5f 	eor	v31.16b, v18.16b, v2.16b
 abc:	4e205929 	cnt	v9.16b, v9.16b
 ac0:	4e2b8400 	add	v0.16b, v0.16b, v11.16b
 ac4:	3ce26a63 	ldr	q3, [x19, x2]
 ac8:	4e205908 	cnt	v8.16b, v8.16b
 acc:	4e2a8421 	add	v1.16b, v1.16b, v10.16b
 ad0:	6e221e2a 	eor	v10.16b, v17.16b, v2.16b
 ad4:	4e205bff 	cnt	v31.16b, v31.16b
 ad8:	4e298400 	add	v0.16b, v0.16b, v9.16b
 adc:	6e231e29 	eor	v9.16b, v17.16b, v3.16b
 ae0:	3ce16a62 	ldr	q2, [x19, x1]
 ae4:	4e288421 	add	v1.16b, v1.16b, v8.16b
 ae8:	4e20594a 	cnt	v10.16b, v10.16b
 aec:	6e231e08 	eor	v8.16b, v16.16b, v3.16b
 af0:	4e3f8400 	add	v0.16b, v0.16b, v31.16b
 af4:	4e205929 	cnt	v9.16b, v9.16b
 af8:	6e301c5f 	eor	v31.16b, v2.16b, v16.16b
 afc:	4e205908 	cnt	v8.16b, v8.16b
 b00:	4e2a8421 	add	v1.16b, v1.16b, v10.16b
 b04:	4e298400 	add	v0.16b, v0.16b, v9.16b
 b08:	4e205bff 	cnt	v31.16b, v31.16b
 b0c:	4e288421 	add	v1.16b, v1.16b, v8.16b
 b10:	4e3f8400 	add	v0.16b, v0.16b, v31.16b
 b14:	4e31b828 	addv	b8, v1.16b
 b18:	4e218400 	add	v0.16b, v0.16b, v1.16b
 b1c:	0e013d01 	umov	w1, v8.b[0]
 b20:	4e31b801 	addv	b1, v0.16b
 b24:	4ea01c08 	mov	v8.16b, v0.16b
 b28:	f90000a1 	str	x1, [x5]
 b2c:	0e013c21 	umov	w1, v1.b[0]
 b30:	f90200a1 	str	x1, [x5, #1024]
 b34:	912000a5 	add	x5, x5, #0x800
 b38:	6b00011f 	cmp	w8, w0
            .......
\end{verbatim}
